# Supplementary material for: Mass-Producing Failures of Multimodal Systems with Language Models
Source: arXiv:2306.12105 source file (2024-03-01)
Supplement: Supplementary file 1 [file extra_clip_results.tex]

\section{Additional quantitative results on CLIP}
\label{sec:additional-quant-results}
